# Supplementary material for: Markov Chain Score Ascent: A Unifying Framework of Variational Inference with Markovian Gradients
Source: arXiv:2206.06295 source file (2022-10-13)
Supplement: Supplementary file 1 [file paretok_additional.tex]

\subsection{Additional Results of Logistic Regression Experiments}

\begin{figure}[H]
  \centering
  \subfloat[Pima]{
    \includegraphics[scale=0.80]{figures/pima_01.pdf}
  }
  \subfloat[Heart]{
    \includegraphics[scale=0.80]{figures/heart_01.pdf}
  }
  \caption{Pareto-\(\widehat{k}\) results of logistic regression problems.
    The solid lines are the median of 100 repetitions while the colored regions are the 80\% empirical percentiles.
  }
\end{figure}

%%% Local Variables:
%%% TeX-master: "master"
%%% End:
